# Supplementary material for: Identify Susceptible Locations in Medical Records via Adversarial Attacks on Deep Predictive Models
Source: arXiv:1802.04822 source file (2018-02-13)
Supplement: Supplementary file 1 [file appendix.tex]

% !TEX root = ./main.tex

\noindent\textbf{Cohort level trade-off}
Figure \ref{fig:fold-1} shows the maximum perturbation and percentage of perturbation under different sparsity control at cohort level. We can see that as regularization increases, the maximum perturbation increases across all observations. Similarly, there is a more clear pattern for perturbation percentage with respect to regularization. A huge penalty would eventually encourage no spots to be changed and end up with failed adversarial records. Figure \ref{fig:fold-1c} indicates whether adversarial is successful, 0 for failure 1 for success respectively, across different regularizations. We can see that the attack generate success adversarial records most of the time.

%\begin{figure}[h!]
%	\centering
%	\vspace{-1em}
%	\includegraphics[width=0.6\columnwidth]{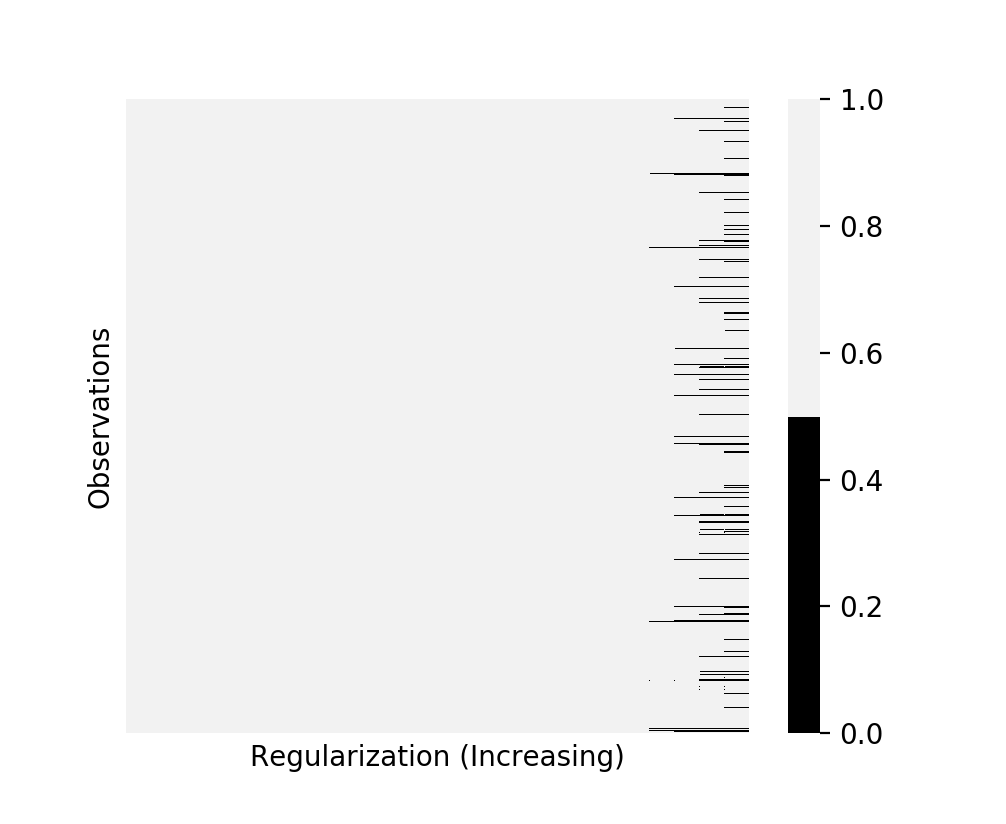}
%	\caption{Success Indicator.}
%	\label{fig:fold-1c}
%\end{figure}

\noindent\textbf{Adversarial results for 1-0 attack} Figure \ref{fig:pop-attack-one} shows the the global maximum perturbation (GMP), global average perturbation (GAP) and global perturbation probability (GPP) at each time-measurement grid for 1-0 attack. Figure \ref{fig:ss-one} shows the susceptibility score for each time-feature grid and overall score for features across 5 folds for 1-0 attack. Table \ref{ss-one} shows the average susceptible score for each feature across 5 folds for 1-0 attack. Figure \ref{fig:sr-one} shows the adversarial assessment for 1-0 attack. We can see that it is harder to perturb a patient from dead to alive compared to the other way around.

%\begin{table}[]
%	\centering
%	\caption{Rank of measurement.}
%	\label{ss-one}\scriptsize
%	\begin{tabular}{|c|c|c|c|}
%		\hline
%		Rank & Measurement & Score & SD   \\ \hline
%		1    & Cre         & 1.95  & 0.46 \\ \hline
%		2    & Na          & 1.48  & 0.21 \\ \hline
%		3    & Lactate     & 0.72  & 0.33 \\ \hline
%		4    & HCO3        & 0.56  & 0.27 \\ \hline
%		5    & PH          & 0.54  & 0.15 \\ \hline
%		6    & Albumin     & 0.54  & 0.23 \\ \hline
%		7    & DBP         & 0.47  & 0.15 \\ \hline
%		8    & Mg          & 0.45  & 0.11 \\ \hline
%		9    & PaCO2       & 0.43  & 0.39 \\ \hline
%		10   & SBP         & 0.40  & 0.15 \\ \hline
%		11   & RR          & 0.38  & 0.14 \\ \hline
%		12   & SPO2        & 0.28  & 0.16 \\ \hline
%		13   & Ca          & 0.25  & 0.08 \\ \hline
%		14   & K           & 0.18  & 0.08 \\ \hline
%		15   & HR          & 0.13  & 0.06 \\ \hline
%		16   & Glc         & 0.13  & 0.11 \\ \hline
%		17   & Platelets   & 0.11  & 0.10 \\ \hline
%		18   & BUN         & 0.09  & 0.03 \\ \hline
%		19   & TEMP        & 0.04  & 0.02 \\ \hline
%	\end{tabular}
%\end{table}
%
